# Supplementary material for: AI Chains: Transparent and Controllable Human-AI Interaction by Chaining Large Language Model Prompts
Source: arXiv:2110.01691 source file (2022-03-17)
Supplement: Supplementary file 1 [file primitive_operation.tex]

%\clearpage
%\newpage
\section{The Full Implementation of Primitive Operations}
\label{sec:appendix-primitive-implement}

%\specialrule{0pt}{1.5pt}{1.5pt}

\begin{table*}[ht]
\fontsize{7.5}{8}\selectfont
%\small
\centering
\begin{subtable}[ht]{ 1\textwidth}
\setlength{\tabcolsep}{3pt}

\begin{tabular}{@{} r | p{0.3\textwidth} | p{0.58\textwidth} | c @{}}
\toprule
\multicolumn{2}{l|}{\textbf{\small{Prompt template}}} & \textbf{\small{Example}} & \textbf{\small{T}}\\
\midrule\midrule
\primTypeTable{Classification}{Assign the input based on limited categories. Most useful for branching logics and validation.}
Instruct &
    \primTemplate{Classify if \primPrefix{cinput1}{\primDescStr{1}} \primPrefix{coutput1}{\primDescStr{2}}.} & 
    \primTemplate{Classify if \primPrefix{cinput1}{the question} \primPrefix{coutput1}{is answerable}.} &
    0
    \\
Input &
    \primRow{cinput1}{\primPrefixStr{1}}{}{(str)} &
    \primRow{cinput1}{question}{What is the square root of banana}{} & \\
output &
    \primRow{coutput1}{\primPrefixStr{2}}{}{\primLLMGen{(str)}} &
    \primRow{coutput1}{is answerable (Yes/No)}{\primLLMGen{No}}{} & \\
\arrayrulecolor{black!100}\bottomrule
\end{tabular}
\subcaption{Primitive for \textbf{examining the given input}, to judge its value (potentially with reasoning), and what to do next.}
\label{table:primitive-exam-context_full}
\end{subtable}

%%%%%%%%%%%%%%%%%%%%%%
\begin{subtable}[ht]{ 1\textwidth}
\setlength{\tabcolsep}{3pt}

\begin{tabular}{@{} r | p{0.3\textwidth} | p{0.58\textwidth} | c @{}}
\toprule
%\multicolumn{2}{l|}{\textbf{Prompt template}} & \textbf{Example} & \textbf{T}\\
%\midrule\midrule

%%%%%%%%%%%%%%%%%%%%%%%%%
%%%%%%%%%%%%%%%%%%%%%%%%%

\primTypeTable{Information Extraction}{Gather some information from the context.}
Instruct &
    \primTemplate{Given \primPrefix{cinput1}{\primDescStr{1}}, extract \primPrefix{coutput1}{\primDescStr{2}}.} & 
    \primTemplate{Given \primPrefix{cinput1}{text}, extract \primPrefix{coutput1}{airport codes for the cities}.} &
    0.2
    \\
Input &
    \primRow{cinput1}{\primPrefixStr{1}}{}{(string)} &
    \primRow{cinput1}{text}{I want to fly from Los Angeles to Miami.}{} & \\
output &
    \primRow{coutput1}{\primPrefixStr{2}}{}{\primLLMGen{(string)}} &
    \primRow{coutput1}{airport codes}{\primLLMGen{LAX, MIA}}{} & \\
\mainrule

%%%%%%%%%%%%%%%%%%%%%%%%%
%%%%%%%%%%%%%%%%%%%%%%%%%

\primTypeTable{Rewriting}{1-1 mapping that changes the input to more machine-readable formats (e.g. json to natural language).}
Instruct &
    \primTemplate{Rewrite \primPrefix{cinput1}{\primDescStr{1}} into \primPrefix{coutput1}{\primDescStr{2}}.} & 
    \primTemplate{Rewrite \primPrefix{cinput1}{the first-person text} into \primPrefix{coutput1}{third-person text}.} &
    0.3
    \\
Input &
    \primRow{cinput1}{\primPrefixStr{1}}{}{(string)} &
    \primRow{cinput1}{first-person text}{I decide to make a movie}{} & \\
output &
    \primRow{coutput1}{\primPrefixStr{2}}{}{\primLLMGen{(string)}} &
    \primRow{coutput1}{third-person text}{\primLLMGen{He decides to make a movie.}}{} & \\
\mainrule

%%%%%%%%%%%%%%%%%%%%%%%%%
%%%%%%%%%%%%%%%%%%%%%%%%%

\primTypeTable{Split Points}{1-N mapping that is particularly useful for splitting contexts.}
Instruct &
    \primTemplate{Split \primPrefix{cinput1}{\primDescStr{1}} into a list of \primPrefix{coutput1}{\primDescStr{2}}.} & 
    \primTemplate{Split \primPrefix{cinput1}{the descriptions on the direction} into a list of \primPrefix{coutput1}{turn-by-turn directions}.} &
    0.3
    \\
Input &
    \primRow{cinput1}{\primPrefixStr{1}}{}{(string)} &
    \primRow{cinput1}{Direction description}{Go south on 95 until you hit Sunrise Blvd, then take it east to US-1 and head south.}{} & \\
output &
    \primRow{coutput1}{\primPrefixStr{2}}{1.}{\primLLMGen{(list of strings)}} &
    \primRow{coutput1}{turn-by-turn directions}{1. \primLLMGen{Drive south on 95.}\newline
        \primLLMGen{2. Turn left onto Sunrise Blvd.}\newline
        \primLLMGen{3. Turn left onto US-1 SE.}}{} & \\
\mainrule
%%%%%%%%%%%%%%%%%%%%%%%%%
%%%%%%%%%%%%%%%%%%%%%%%%%

\primTypeTable{Compose Points}{N-1 mapping, the reverse operation of decomposition; merge multiple results back.}
Instruct &
    \primTemplate{Write one \primPrefix{coutput1}{\primDescStr{1}} to cover all the \primPrefix{cinput1}{\primDescStr{2}}.} & 
    \primTemplate{Write one \primPrefix{coutput1}{review} to cover all the \primPrefix{cinput1}{restaurant name} and \primPrefix{cinput2}{notes}.} &
    0.5
    \\
Input &
    \primRow{cinput1}{\primPrefixStr{1}}{}{(list of strings)} &
    \primRow{cinput1}{Restaurant name}{The Blue Wharf}{}\newline
    \primRow{cinput2}{Short notes}{1. Lobster great; 2.noisy; 3.service polite}{} & \\
output &
    \primRow{coutput1}{\primPrefixStr{2}}{}{\primLLMGen{(string)}} &
    \primRow{coutput1}{Review}{\primLLMGen{The place is great if you like lobster. The noise level} \newline
    \primLLMGen{is a little high, but the service is polite.}}{} & \\

\arrayrulecolor{black!100}\bottomrule
\end{tabular}
\subcaption{Primitives for \textbf{reorganizing the given input}, and re-format it by parsing and expressing them in different ways.}
\label{table:primitive-format-context_full}
\end{subtable}

%%%%%%%%%%%%%%%%%%%%%%
\begin{subtable}[ht]{ 1\textwidth}
\setlength{\tabcolsep}{3pt}

\begin{tabular}{@{} r | p{0.3\textwidth} | p{0.58\textwidth} | c @{}}
\toprule
%\multicolumn{2}{l|}{\textbf{Prompt template}} & \textbf{Example} & \textbf{T}\\
%\midrule\midrule

%%%%%%%%%%%%%%%%%%%%%%%%%
%%%%%%%%%%%%%%%%%%%%%%%%%

\primTypeTable{Factual Query}{Ask the model for a fact.}
Instruct &
    \primTemplate{Given \primPrefix{cinput1}{\primDescStr{1}}, find \primPrefix{coutput1}{\primDescStr{2}}.} & 
    \primTemplate{Given \primPrefix{cinput1}{the US state}, find \primPrefix{coutput1}{the population}.} &
    0.3
    \\
Input &
    \primRow{cinput1}{\primPrefixStr{1}}{}{(string)} &
    \primRow{cinput1}{US state}{Washington}{} & \\
output &
    \primRow{coutput1}{\primPrefixStr{2}}{}{\primLLMGen{(string)}} &
    \primRow{coutput1}{Population}{\primLLMGen{7.6 million}}{} & \\
\mainrule

%%%%%%%%%%%%%%%%%%%%%%%%%
%%%%%%%%%%%%%%%%%%%%%%%%%

\primTypeTable{Generation}{Ask the model to do some creative “hallucination” on the input.}
Instruct &
    \primTemplate{Given \primPrefix{cinput1}{\primDescStr{1}}, create \primPrefix{coutput1}{\primDescStr{2}}.} & 
    \primTemplate{Given \primPrefix{cinput1}{the topic}, create \primPrefix{coutput1}{a two-sentence horror story}.} &
    0.7
    \\
Input &
    \primRow{cinput1}{\primPrefixStr{1}}{}{(string)} &
    \primRow{cinput1}{topic}{Breakfast}{} & \\
output &
    \primRow{coutput1}{\primPrefixStr{2}}{}{\primLLMGen{(string)}} &
    \primRow{coutput1}{two-sentence horror story}{\primLLMGen{He always stops crying when I pour} \newline
    \primLLMGen{the milk on his cereal. I just have to remember not to let him}\newline 
    \primLLMGen{see his face on the carton.}}{} & \\
\mainrule

%%%%%%%%%%%%%%%%%%%%%%%%%
%%%%%%%%%%%%%%%%%%%%%%%%%

\primTypeTable{Ideation}{Ask the model for a list of ideas or examples.}
Instruct &
    \primTemplate{Given \primPrefix{cinput1}{\primDescStr{1}}, the following is a list of \primPrefix{coutput1}{\primDescStr{2}}.} & 
    \primTemplate{Given \primPrefix{cinput1}{the interviewee}, the following is a list of \primPrefix{coutput1}{interview questions}.} &
    0.7
    \\
Input &
    \primRow{cinput1}{\primPrefixStr{1}}{}{(string)} &
    \primRow{cinput1}{Interviewee}{A science fiction author}{} & \\
output &
    \primRow{coutput1}{\primPrefixStr{2}}{1.}{\primLLMGen{(list of strings)}} &
    \primRow{coutput1}{Interview questions}{1. \primLLMGen{What's your favorite sci-fi book?}\newline
        \primLLMGen{2. Who inspired you to start writing books?}}{} & \\
\arrayrulecolor{black!100}\bottomrule
\end{tabular}
\subcaption{Primitives for \textbf{gathering additional clues from LLMs}, when the desired output is too longer or too diverse.}
\label{table:primitive-add-info_full}
\end{subtable}
\caption{We design a list of primitive building blocks, each with default prompting templates and temperatures, and group them by their intended objectives. Examples are taken from \url{https://beta.openai.com/examples}.
}
\label{table:primitive_full}
\vspace{-10pt}
\end{table*}
