# Supplementary material for: AI Chains: Transparent and Controllable Human-AI Interaction by Chaining Large Language Model Prompts
Source: arXiv:2110.01691 source file (2022-03-17)
Supplement: Supplementary file 2 [file viz_result.tex]

when it's all information involved
\begin{comment}
# correct
('On [encoding: x], [scale type: log] conflicts with [data type: nominal].
How to fix: On [encoding: x], remove [scale type: log] or change [data type: nominal] to [data"encoding": {\n    
"x": {"field": "Origin", "bin": true, "type": "nominal"},
"y": {"field": "Horsepower", "type": "quantitative", "aggregate": "mean"}\n}\}',)

# incorrect
('On [encoding: x], [scale type: log] conflicts with [data type: nominal].
How to fix: On [encoding: x], remove [scale type: log].\n', 
["x": {"field": "Origin", "aggregate": "sum", "type": "nominal"} <|INCLUDE|> ["x": {"field": "Origin", "type[y: quantitative].}

# incorrect
('On [encoding: x] , [mark type: bar] is invalid.
How to fix: Replace [mark type: bar] with [mark type: point].\n', 
' \n<|-- bar<|-- point')

# incorrect
('On [encoding: x], [scale type: log] is invalid, when [data type: quantitative].
How to fix: Replace [scale type: log] with [scale type: linear].\n', 
' \n<|--scale type: log-->\n<|--scale type: linear-->')

# incorrect
('On [encoding: x] , [mark: bar] is invalid, when having [x: quantitative] and [y: quantitative].\nHow to fix: Replace [bin: true] with [size: xxx].',)
\end{comment}

when it's nothing

\begin{comment}
%('["x": {"field": "Origin","type": "nominal","scale": {"type": "log"}} <|PERTURB|> "x": {"field":"Origin","type": "nominal"}],"scale": {"type": "log"}}]',)

%('["x": {"field": "Origin", "bin": true, "type": "nominal"} <|PERTURB|> "x": {"field": "Origin", "type": "nominal"}]"}]',)

incorrect
%('["x": {"field": "Horsepower","type": "quantitative"} <|PERTURB|> "x": {"field": "Horsepower","type": "quantitative"}]}]',)

incorrect
%('["x": {"field": "Acceleration","type": "quantitative"} <|PERTURB|> "x": {"field": "Acceleration","type": "quantitative"}]"}]',)

incorrect
%('["x": {"field": "Origin", "bin": true, "type": "nominal"} <|PERTURB|> "x": {"field": "Origin", "type": "nominal"}]"}]',)

\end{comment}

('On [encoding: x], [scale type: log] conflicts with [data type: nominal].\nHow to fix: On [encoding: x], remove [scale type: log].\n', ' ["x": {"field": "Origin", "aggregate": "sum", "type": "nominal"} <|INCLUDE|> ["x": {"field": "Origin", "type[y: quantitative].\nB) [encoding: x] has [bin: True], [data type: nominal].\nC) [encoding: y] has [data type: quantitative], [aggregate: mean].\nRules: 1) [mark type: bar] is invalid, when having [x: quantitative] and [y: quantitative].\n2) [encoding: size] is invalid, when having [data type: quantitative].\n3) [scale type: log] is invalid, if it does not have [data type: quantitative].\n4) [scale type: log] is invalid, when having [scale zero: True].\n5) [mark type: line] is invalid, if it does not have both [x] and [y].\n6) [bin: True] is invalid, when having [aggregate]..\n7) [bin: True] is invalid, when it does not have [data type: quantitative]..\n8) [aggregate: sum] is invalid, when having [data type: nominal]..\nValid/Invaid: On [encoding: x], [bin: true] conflicts with [data type: nominal].\nHow to fix: Remove [bin: True] from [encoding: x].\n', ' ["x": {"field": "Origin", "bin": true, "type": "nominal"} <|PERTURB|> "x": {"field": "Origin", "type": "nominal"}]\n')

('On [encoding: x] , [mark type: bar] is invalid.\nHow to fix: Replace [mark type: bar] with [mark type: point].\n', ' \n<|-- bar<|-- point')

('On [encoding: x], [scale type: log] is invalid, when [data type: quantitative].\nHow to fix: Replace [scale type: log] with [scale type: linear].\n', ' \n<|--scale type: log-->\n<|--scale type: linear-->')

('On [encoding: x] , [mark: bar] is invalid, when having [x: quantitative] and [y: quantitative].\nHow to fix: Replace [bin: true] with [size: xxx].',)
